# Supplementary material for: STEMM: Self-learning with Speech-text Manifold Mixup for Speech Translation
Source: arXiv:2203.10426 source file (2022-03-20)
Supplement: Supplementary file 1 [file appendix.tex]

\section{Statistics of all datasets}
\label{sec:statistics}
\input{Tables/data.tex}
